# Supplementary material for: Exploration of the Parameter Space in Macroeconomic Agent-Based Models
Source: arXiv:2111.08654 source file (2022-08-05)
Supplement: Supplementary file 1 [file appx_breakdown.tex]

\subsection{Breakdown at EU-FE Transition}

\begin{itemize}
    \item \textbf{Observation} \\
    Breakdown of economy is accommodated with a peak in wages on a firm level, high rate of bankrupt firms and growing number of firms with zero production. It seems that in every endogenous crisis cycle more firms go bankrupt than revived firms, which results in a dead economy with high unemployment.
    \item \textbf{Investigation} (parameter EC 1 are compared to parameter phase 3) \\
    A single firm goes bankrupt in the following chain of events
    \begin{itemize}
        \item Loan interest rate starts to increase slowly
        \item this causes that firms with $A[i] \approx \theta$ go bankrupt
        \item this initiates a negative feedback loop such that the loan interest rate continues to increase and firms with average $A[i]$ start to go bankrupt due to a strong decrease of $PROFIT[i]$.
    \end{itemize}
    Why doesn't this happen in the EC case?
    \begin{itemize}
        \item Difference between the two parameter sets are $\theta_{EC} < \theta_{phase}$ and $\rho^*_{EC} = \frac{\rho^*_{phase}}{2} $
        \item In every time step $\rho_m$ increase if total debt is bigger than zero, which is always true. The important equations are \\
        \begin{equation}
            \rho = \rho^* + FACPI * \pi_{target} + \phi_{\pi} * ( \pi_{avg} - \pi_{target} ) + 0 * \phi_e * gsl_sf_log((1.-u_{avg})/tmp)
        \end{equation}
        \begin{equation}
            if(debt_{tot} > 0.) \, \, \rho_m += (1.-f)*deftot / debt_{tot} 
        \end{equation}
        Since $\rho_m$ is per default higher with the phase parameters because $\rho_m = \rho$, the peak in loan interest rate is fostered. Additionally, $debt_{tot, EC} \gg debt_{tot, phase}$ therefore the increase in $\rho_m$ is bigger. Deftot increase if firms go bankrupt and revive again. Since this happens with the phase parameter more often, the $\rho_m$ increase is even higher. 
        \item Therefore, peaks in $\rho_m$ happen with the phase parameter more often throughout the simulation therefore it is not possible to preserve the endogenous crisis fluctuation but rather drift off into the FU phase.
        \item By increasing $\theta$ we end up in a FE phase, because the higher $\theta$ the less bankruptcies occur, which inhibits the negative feedback loop initiated by $\rho_m$
    \end{itemize}
\end{itemize}

\subsection{FE-RU / EC-RU Transition}

\begin{itemize}
    \item \textbf{Observation} \\
    If we start in the EC or in the FE phase, and increase $\rho^*$ we end up in the RU phase. According to the explanation above, with increasing $\rho^*$ the height of the peaks should increase which should end up in a breakdown of the economy due to the negative feedback loop of bankruptcies.
    \item \textbf{Investigation} \\
    We see that if $\rho^*$ is bigger than the inflation rate, there is a negative feedback loop due to a rise in unemployment causing inflation rate to decrease causing an in crease in unemployment. Additionally, due to the reaction of firms to interest rates
    \begin{equation}
        \Gamma = max(\alpha_{\Gamma} * (\rho^l_{avg}-\pi_{used}),\Gamma_0)
    \end{equation}
    the demand for debt decreases. Reasonably, firms are afraid from taking debt and rather fire labor which causes the unemployment rate to rise.
\end{itemize}
