# Supplementary material for: Exploration of the Parameter Space in Macroeconomic Agent-Based Models
Source: arXiv:2111.08654 source file (2022-08-05)
Supplement: Supplementary file 2 [file appx_exponentials.tex]

In order to ensure that the implementation of the Hessian estimation and approximation are correct, we analyze the analytically tractable problem of fitting polynomials. Consider the function
\begin{equation}\label{eq:polynomial_function}
    f(x, \Theta) = \sum_{n=0}^N p_n x^n,
\end{equation}
with parameter vector $\Theta=[p_0, \dots, p_N]$ and $x\in[0,1]$.

\subsection{Derivation of the analytical Hessian}
\noindent We consider the loss function of Eq. \eqref{eq:loss_function} in the absence of noise ($N_s=1$), and for only one variable ($N_k=1$):
\begin{equation}\label{eq:polynomial_loss_function}
\mathcal{L}(\Theta) = \frac{1}{2N}\sum_{N}\left(f(x_n,\Theta) - f(x_n,\Theta^\star)\right)^2,
\end{equation}
as a simplification of the original noise function that will allow us to demonstrate the feasibility of our numerical estimates. 
From this we can then derive the Hessian matrix that will be numerically approximated as
\begin{equation}
H_{i,j}^{\mathcal{L}} \equiv \frac{d^2\mathcal{L}}{d\Theta_i d\Theta_j}
\end{equation}
at the point $\Theta^\star$ by taking the second derivative at this point, leading to
\begin{equation}\label{eq:polynomial_first_order_approx}
\frac{d^2\mathcal{L}(\Theta)}{d\Theta_i d\Theta_j} = \frac{1}{N
}\sum_{N}\frac{df(x_n, \Theta^\star)}{d\Theta_i}\frac{df(x_n, \Theta^\star)}{d\Theta_j},
\end{equation} 

\noindent Analytically, the Hessian matrix of this system is the Hilbert matrix, such that $H^\star_{i,j}=\frac{2}{i+j+1}$. This can be seen by considering the vector of $\frac{df(x_n, \Theta^\star)}{d\Theta_i}$, namely the Jacobian, $J = [1, x, x^2, \dots, x^N]^\top$, which leads us to the analytical Hessian Matrix $H^\star$ (here for the case of $N=4$)
\begin{equation}
    H^\star = \frac{1}{N}\sum_{N}\left[\begin{array}{cccc}
        1 & x_n & x_n^2 & x_n^3 \\
        x_n & x_n^2 & x_n^3 & x_n^4\\
        x_n^2 & x_n^3 & x_n^4 & x_n^5\\
        x_n^3 & x_n^4 & x_n^5 & x_n^6\\
    \end{array}\right] \xrightarrow[]{N\to\infty}
    \left[\begin{array}{cccc}
        1       & {1}/{2} & {1}/{3} & {1}/{4} \\
        {1}/{2} & {1}/{3} & {1}/{4} & {1}/{5}\\
        {1}/{3} & {1}/{4} & {1}/{5} & {1}/{6}\\
        {1}/{4} & {1}/{5} & {1}/{6} & {1}/{7}\\
    \end{array}\right]
\end{equation}
which converges to the Hilbert matrix. 

\subsection{Numerical results}
Given confirmation that both the implemented $\mathcal{O}(N^2)$ numerical approximation and the first-order approximation (Eq. \eqref{eq:polynomial_first_order_approx}) converge to the Hilbert matrix, we can study their convergence properties as functions of the amount of data and the number of variables supplied to the algorithms.

\begin{figure}[htb!]
    \centering
    \includegraphics[width=\textwidth]{figures/fig_polynomials_convergence_vs_data_val.pdf}
    \caption{The number of unique entries $(i,j)$ where ${\hat{H}^{\mathcal{L}}_{i,j}} / {H^\star_{i,j}} - 1 > \epsilon$ as a function of the number of data-points provided. 
    }
    \label{fig:polynomial_convergence_T}
\end{figure}

\subsection{Introducing Noise}
To further study the convergence times in the presence of distorting noise, we consider an adapted polynomial problem
\begin{equation}\label{eq:polynomial_function_noise}
    f(x, \Theta) = \sum_{n=0}^N p_n x^n + \xi,
\end{equation}
where $\xi\sim N(0,\sigma)$ is a normally distributed random variable that will distort the outcome of the polynomial. Since $\xi$ is independent of the parameters and the data, this results in maintaining the Hilbert matrix as the true Hessian matrix while merely distorting the data.

The logic of the idea:
\begin{itemize}
    \item Set a given $x_0$ using $seed_{init}$
    \item Compute target via $f(x_0, \Theta)$
    \item For every seed $s$ we compute:
    $f(x_0, \Theta^\star) + \xi_s$
    \item Consequence: if we take $N_s$ seeds then take the Hessian over the seeds something of the form 
    $\frac{1}{N_s}\sum_{s}f(x_0, \Theta) + \xi_s \xrightarrow{N_s\to\infty} f(x_0)$ should happen
\end{itemize}

\begin{figure}[htb!]
    \centering
    \includegraphics[width=\textwidth]{example-image-b}
    \caption{Heatmap for the number of datapoints (number of seeds by data length $T$) necessary for the number of elements $(i,j)$ where difference $\hat{H}^{\mathcal{L}}_{i,j} / {H^\star_{i,j}} - 1 < \epsilon$, to be smaller than an small deviation $\epsilon=10^{-3}$ as function of the number of parameters and the standard deviation noise term, $\sigma$. For this instance we work with additional datapoints in $T=10$ size intervals
    }
    \label{fig:polynomial_convergence_T}
\end{figure}
