# Supplementary material for: Exploration of the Parameter Space in Macroeconomic Agent-Based Models
Source: arXiv:2111.08654 source file (2022-08-05)
Supplement: Supplementary file 3 [file appx_kl_derivatives.tex]

\section{Kullback-Leibler Divergence}
In place of comparing the time-series of the observable outputs directly (as done in Eq. \ref{eq:square_loss}), we can instead compare their distributions by the Kullback-Leibler divergence. The Kullback-Leibler divergence compares the probability density functions of two candidate series. Define $P(X|\Phi)$ as the PDF of observable $X$ generated by the parameter set $\Phi$, similarly, define $P(X|\Phi+\delta)$ to be the PDF of observable $X$ generated by an alternate parameter set $\Phi+\delta$. The Kullback-Leibler divergence between these two functions is defined by
\begin{equation}\label{eq:kl_divergence}
	D_{KL}(P(X|\Phi),~P(X|\Phi+\delta)) = \sum_{x\in X} P(x|\Phi)\log\left(\frac{P(x|\Phi)}{P(x|\Phi+\delta)}\right),
\end{equation}

Unfortunately, the KL divergence is not a metric, as it is asymmetric ($D_{KL}(P(X|\Phi),~P(X|\Phi+\delta))\neq D_{KL}(P(X|\Phi+\delta),~P(X|\Phi))$) and does not obey the triangle inequality. This can be addressed by symmetrising the KL divergence,
\begin{equation}
	D_{sKL}(P(X|\Phi),~P(X|\Phi+\delta)) = 	D_{KL}(P(X|\Phi),~P(X|\Phi+\delta)) + D_{KL}(P(X|\Phi+\delta),~P(X|\Phi)),
\end{equation}
which leads to a non-zero metric for the distance between the two distributions (zero when $\delta=0$, and positive otherwise). Regardless of our choice in formulation, we seek the Hessian matrix
\begin{equation}
	H_{i,j}^{\mathcal{L}}(\Phi) := \left. \frac{d^2\mathcal{L}(\Phi, \delta)}{d\log\Phi_i d\log\Phi_j} \right|_{\delta = 0}
\end{equation}
to determine the model's sloppiness and exploit this for our algorithm. To determine this for the symmetrized case, we proceed with each individual direction first, before combining them.

\subsection{Hessian matrix of $D_{KL}(P(X|\Phi),~P(X|\Phi+\delta))$}
Let $\frac{\partial}{\partial \Phi_j} = \partial_j$, such that we can write the first derivative as
\begin{align}
	\partial_j D_{KL}(P(X|\Phi),~P(X|\Phi+\delta)) &= \sum_{x\in X} \partial_j P(x|\Phi)\log\left(\frac{P(x|\Phi)}{P(x|\Phi+\delta)}\right)\\
	&= \sum_{x\in X} P(x|\Phi) \partial_j \log\left(\frac{P(x|\Phi)}{P(x|\Phi+\delta)}\right)\\
	&= \sum_{x\in X} P(x|\Phi) \frac{P(x|\Phi+\delta)}{P(x|\Phi)} \partial_j \left(\frac{P(x|\Phi)}{P(x|\Phi+\delta)}\right)\\
	&= -\sum_{x\in X} P(x|\Phi+\delta) \frac{P(x|\Phi)\partial_j P(x|\Phi+\delta)}{P(x|\Phi+\delta) ^ 2}\\
	&= -\sum_{x\in X} P(x|\Phi) \frac{\partial_j P(x|\Phi+\delta)}{P(x|\Phi+\delta)}\\
	&= -\sum_{x\in X} P(x|\Phi) \partial_j \log P(x|\Phi+\delta),
\end{align}
where $\partial_j P(x|\Phi) = 0$. Moving to the second derivative $\partial_i$ we have
\begin{align}
	\partial_i \partial_j D_{KL}(P(X|\Phi),~P(X|\Phi+\delta)) &= \partial_i \left[-\sum_{x\in X} P(x|\Phi) \frac{\partial_j P(x|\Phi+\delta)}{P(x|\Phi+\delta)}\right]\\
	&= -\sum_{x\in X} P(x|\Phi) \partial_i \frac{\partial_j P(x|\Phi+\delta)}{P(x|\Phi+\delta)}\\
	&= -\sum_{x\in X} P(x|\Phi) \left[\frac{\partial_i \partial_j P(x|\Phi+\delta)}{P(x|\Phi+\delta)} -\frac{ \partial_j P(x|\Phi+\delta)\partial_i P(x|\Phi+\delta)}{P(x|\Phi+\delta)^2}\right],
\end{align}
where we now make the following observation: since we are evaluating the second derivative at the point $\delta=0$, we can substitute the following
\begin{equation}\label{eq:second_zero}
	-\sum_{x\in X} P(x|\Phi) \frac{\partial_i \partial_j P(x|\Phi+\delta)}{P(x|\Phi+\delta)} \stackrel{\delta=0}{=} -\sum_{x\in X} \partial_i \partial_j P(x|\Phi) = \partial_i \partial_j\left(-\sum_{x\in X} P(x|\Phi)\right) = \partial_i \partial_j\left(-1\right) = 0,
\end{equation}
which leads us to the resulting equation (noting that $\delta=0$)
\begin{align}
	\partial_i \partial_j D_{KL}(P(X|\Phi),~P(X|\Phi+\delta)) &= \sum_{x\in X} P(x|\Phi) \frac{ \partial_j P(x|\Phi)\partial_i P(x|\Phi)}{P(x|\Phi)^2} \\
	&= \sum_{x\in X} P(x|\Phi) \partial_j \log P(x|\Phi) \partial_i \log P(x|\Phi),
\end{align}
which is the Fisher information matrix.

\subsection{Hessian matrix of $D_{KL}(P(X|\Phi+\delta),~P(X|\Phi))$}
Turning now to the reverse case, we follow the same procedure as before:
\begin{align}
	\partial_j D_{KL}(P(X|\Phi+\delta), ~P(X|\Phi)) &= \sum_{x\in X} \partial_j P(x|\Phi+\delta)\log\left(\frac{P(x|\Phi+\delta)}{P(x|\Phi)}\right)\\
	&= \sum_{x\in X} \log\left(\frac{P(x|\Phi+\delta)}{P(x|\Phi)}\right) \partial_j P(x|\Phi+\delta) + \sum_{x\in X} P(x|\Phi) \partial_j\left(\frac{P(x|\Phi+\delta)}{P(x|\Phi)}\right)\\
	&= \sum_{x\in X} \log\left(\frac{P(x|\Phi+\delta)}{P(x|\Phi)}\right) \partial_j P(x|\Phi+\delta) + \underbrace{\partial_j \sum_{x\in X} P(x|\Phi+\delta)}_{\textrm{Equals 0}}\\
	&= \sum_{x\in X} \log\left(\frac{P(x|\Phi+\delta)}{P(x|\Phi)}\right) \partial_j P(x|\Phi+\delta),
\end{align}
from this we now turn to the second derivative
\begin{align}
	\partial_i \partial_j D_{KL}(P(X|\Phi),~P(X|\Phi+\delta)) &= \partial_i \left[\sum_{x\in X} \log\left(\frac{P(x|\Phi+\delta)}{P(x|\Phi)}\right) \partial_j P(x|\Phi+\delta)\right]\\
	&= \sum_{x\in X} \partial_i \left[\log\left(\frac{P(x|\Phi+\delta)}{P(x|\Phi)}\right) \partial_j P(x|\Phi+\delta)\right]\\
	&= \sum_{x\in X} \frac{\partial_i P(x|\Phi+\delta) \partial_j P(x|\Phi+\delta)}{P(x|\Phi+\delta)} + \underbrace{\sum_{x\in X} \log\left(\frac{P(x|\Phi+\delta)}{P(x|\Phi)}\right) \partial_i \partial_j P(x|\Phi+\delta)}_{\textrm{Equals to 0 for }\delta=0}\\
	&= \sum_{x\in X} P(x|\Phi)\frac{\partial_i P(x|\Phi) \partial_j P(x|\Phi)}{P(x|\Phi)^2} \quad\quad\textrm{for }\delta=0\\
	&=\sum_{x\in X} P(x|\Phi) \partial_i \log P(x|\Phi) \partial_j \log P(x|\Phi),
\end{align}
Thus we find that regardless of the direction of the KL divergence, the second derivative is always equal to the Fisher Information Matrix. This is beneficial for us as it only requires us to calculate the first derivatives, thus requiring only $\mathcal{O}(N)$ calculations.

\subsection{Hessian matrix in the Symmetrized Case}
Following the previous two sections, the Hessian matrix for the symmetrized KL-divergence is trivially equal to twice the Fisher Information Matrix:
\begin{align}
	\partial_i\partial_jD_{sKL}(P(X|\Phi),~P(X|\Phi+\delta)) &= \partial_i\partial_j\left[D_{KL}(P(X|\Phi),~P(X|\Phi+\delta)) + D_{KL}(P(X|\Phi+\delta),~P(X|\Phi))\right]\\
	&= \partial_i\partial_jD_{KL}(P(X|\Phi),~P(X|\Phi+\delta)) + \partial_i\partial_jD_{KL}(P(X|\Phi+\delta),~P(X|\Phi))\\
	&= 2\sum_{x\in X} P(x|\Phi) \partial_i \log P(x|\Phi) \partial_j \log P(x|\Phi)
\end{align}

\subsection{Integrating the KL-divergence into the Loss function}
The $D_{sKL}$ is a non-negative metric describing the difference between two distributions. For identical distributions it takes value 0, and for non-overlapping distributions it is infinite (i.e. $P(x|\Phi+\delta)=0$, $\forall x\in X$ where $P(x|\Phi)>0$). 
For small changes $\delta$, we expect there to be significant overlap, nonetheless, we normalise the distributions to have mean 0, and also consider their mean in the loss-function:

\begin{equation}\label{eq:loss_kl}
	\mathcal{L}(\Phi, \delta) = \frac{1}{2 S K}\sum_{s}\sum_{k} D_{KL}(P({y_{s,k}}|\Phi),~P(y_{s,k}|\Phi+\delta)),
\end{equation}
which leads to a Hessian matrix
\begin{align}
	H_{i,j}^{\mathcal{L}}(\Phi) &=\partial_i\partial_j\mathcal{L}(\Phi, \delta)\\
	&= \frac{1}{2 S K}\sum_{s}\sum_{k} \partial_i\partial_j D_{KL}(P({y_{s,k}}|\Phi),~P(y_{s,k}|\Phi+\delta))\\
	&=\frac{1}{2 S K}\sum_{s}\sum_{k} \sum_{x\in y_{s,k}} P(x|\Phi) \partial_i \log P(x|\Phi) \partial_j \log P(x|\Phi),
\end{align}

\noindent This formulation raises some numerical questions:
\begin{enumerate}
	\item How to set the bounds and bins for an unbounded observable, especially in the presence of spikes?
	\item 
\end{enumerate}
