# Supplementary material for: Exploration of the Parameter Space in Macroeconomic Agent-Based Models
Source: arXiv:2111.08654 source file (2022-08-05)
Supplement: Supplementary file 4 [file appx_loss_functions.tex]

This appendix shows the loss-functions that have been tested, as well as the approximations of their corresponding Hessian matrices (Fisher Information Matrices). In terms of notation, parameter set $\Theta$ generates a time-series realization $y(\Theta)_{s,k,t}$ of $k\in\{1,\dots,N_K\}$ variables over $t\in\{1,\dots,T\}$ periods using the random seeds $s\in\{1,\dots,N_S\}$. We define $\Theta^\star$ as the parameter set that generates the \textit{target} realization. We also introduce $\alpha=(s,k,t)$ to simplify subscripts.

\subsection{The Mean Squared Loss}
    \begin{equation}\label{eq:loss_sqr}
    \mathcal{L}^{sqr}(\Theta) = \frac{1}{2N_S N_K T}\sum_{s}^{N_S}\sum_{k}^{N_K}\sum_{t}^{T}\left(\frac{y_{s, k, t}(\Theta) - y_{s, k, t}(\Theta^\star)}{\norm{y_{s,k}(\Theta^\star)}}\right)^2,
    \end{equation}
    where $\norm{\cdot}$ is a normalization such as the mean, the maximum or the standard deviation. At the optimum, this loss function equates to zero. The Hessian at $\Theta^\star$ can be derived as follows:
    \begin{equation}
    H_{i,j}^{\mathcal{L}^{sqr}} \equiv \frac{d^2\mathcal{L}(\Theta)}{d\log\Theta_i d\log\Theta_j}
    \end{equation}
    Let $x_\alpha = (y_\alpha(\Theta) - y_\alpha(\Theta^\star))/\norm{y_\alpha(\Theta^\star)}$. Then
    \begin{eqnarray}
    \frac{d\mathcal{L}(\Theta^\star)}{d\log\Theta_id\log\Theta_j}\bigg|_{\Theta=\Theta^\star} &=& \frac{1}{2N_S N_K T}\sum_{\alpha} \frac{d}{d\log\Theta_i}\frac{d}{d\log\Theta_j}x_\alpha^2, \\
    &=& \frac{1}{N_S N_K T}\sum_{\alpha} \frac{d}{d\log\Theta_i}\left(\frac{x_\alpha}{\norm{y_\alpha(\Theta^\star)}}\frac{dy_{\alpha}(\Theta^\star)}{d\log\Theta_j}\right), \\
    &=& \frac{1}{N_S N_K T}\sum_{\alpha}\frac{1}{\norm{y_\alpha(\Theta^\star)}^2} \frac{dy_{\alpha}(\Theta^\star)}{d\log\Theta_i}\frac{dy_{\alpha}(\Theta^\star)}{d\log\Theta_j},
    \end{eqnarray}
    where the second order terms vanish when we evaluate the Hessian at the minimum $\Theta^\star$.
    
\subsection{The Mean Squared Percentage Error}
    \begin{equation}\label{eq:loss_sqr}
    \mathcal{L}^{sqrperc}(\Theta) = \frac{1}{N_S N_K T}\sum_{s}^{N_S}\sum_{k}^{N_K}\sum_{t}^{T}\left(1 - \frac{y_{s, k, t}(\Theta)}{y_{s, k, t}(\Theta^\star)}\right)^2,
    \end{equation}
    where the loss at the optimum is equal to zero. There is a danger here that the realization $y(\Theta^\star)_{s,k,t}=0$, which would generate an infinite value. The Hessian is derived as follows:
    \begin{equation}
    H_{i,j}^{\mathcal{L}^{sqrperc}} \equiv \frac{d^2\mathcal{L}(\Theta)}{d\log\Theta_i d\log\Theta_j}
    \end{equation}
    Let $x_\alpha = 1 - y_\alpha(\Theta) / y_\alpha(\Theta^\star)$. Then
    \begin{eqnarray}
    \frac{d\mathcal{L}(\Theta^\star)}{d\log\Theta_id\log\Theta_j}\bigg|_{\Theta=\Theta^\star} &=& \frac{1}{2N_S N_K T}\sum_{\alpha} \frac{d}{d\log\Theta_i}\frac{d}{d\log\Theta_j}x_\alpha^2, \\
    &=& \frac{1}{N_S N_K T}\sum_{\alpha} \frac{d}{d\log\Theta_i}\left(\frac{-x_\alpha}{y_\alpha(\Theta^\star)}\frac{dy_\alpha(\Theta^\star)}{d\log\Theta_j}\right), \\
    &=& \frac{1}{N_S N_K T}\sum_{\alpha}\frac{1}{y_\alpha(\Theta^\star)^2}\frac{dy_{\alpha}(\Theta^\star)}{d\log\Theta_i}\frac{dy_{\alpha}(\Theta^\star)}{d\log\Theta_j},
    \end{eqnarray}
    
\subsection{The Mean Cosh Loss}
    \begin{equation}\label{eq:loss_sqr}
    \mathcal{L}^{cosh}(\Theta) = \frac{1}{N_S N_K T}\sum_{s}^{N_S}\sum_{k}^{N_K}\sum_{t}^{T}\log\left(\cosh\left(y(\Theta)_{s, k, t} - y(\Theta^\star)_{s, k, t}\right)\right),
    \end{equation}
    where the loss at the optimum is equal to zero. There is a danger here that the realization $y(\Theta^\star)_{s,k,t}=0$, which would generate an infinite value. 
    
\subsection{The Mean Log Absolute Loss}
    \begin{equation}\label{eq:loss_sqr}
    \mathcal{L}^{labs}(\Theta) = \frac{-1}{N_S N_K T}\sum_{s}^{N_S}\sum_{k}^{N_K}\sum_{t}^{T}\log\left(\left|\frac{y(\Theta)_{s, k, t} - y(\Theta^\star)_{s, k, t}}{\norm{y_{s,k}}}\right|\right),
    \end{equation}

In the case of the squared loss and the absolute percentage error, the loss equals zero at the optimum. Meanwhile, for the log absolute loss function, the loss function converges to infinity at the optimum.

\begin{equation}\label{eq:loss_function}
\mathcal{L}(\Theta) = \frac{1}{2N_S N_K T}\sum_{s}^{N_S}\sum_{k}^{N_K}\sum_{t}^{T}\log\left(\left|\frac{y(\Theta)_{s, k, t} - y(\Theta^\star)_{s, k, t}}{\norm{y_{s,k}}}\right|\right),
\end{equation}
where $||\cdot||$ is a norm on $y_{s,k}$ such as the mean. We now define:
\begin{eqnarray}
\alpha&=&(s,k,t) \\
x_\alpha &=& \frac{y(\Theta)_\alpha - y(\Theta^\star)_\alpha}{\norm{y_\alpha}} \\
g(x_\alpha) &=& \begin{cases}
-1 & \textrm{for } x_\alpha < 0, \\
1 & \textrm{otherwise}
\end{cases}
\end{eqnarray}
we can now simplify the loss to
\begin{equation}\label{eq:loss_function_simple}
\mathcal{L}(\Theta) = \frac{1}{2N_S N_K T}\sum_{\alpha}\log \abs{x_\alpha}
\end{equation}

\subsection{The Hessian Matrix}
The Hessian matrix is defined as the matrix of second derivatives
\begin{equation}
H_{i,j}^{\mathcal{L}} \equiv \frac{d^2\mathcal{L}(\Theta)}{d\log\Theta_i d\log\Theta_j}
\end{equation}
The derivative is taken with respect to $\log\Theta_i$ to account for different order of magnitudes.
To derive the Hessian matrix of our loss at a target point $\Theta^\star$ we compute:
\begin{equation}
\frac{d\mathcal{L}(\Theta^\star)}{d\log\Theta_id\log\Theta_j} = \frac{1}{N_S N_K T}\sum_{\alpha} \frac{d}{d\log\Theta_i}\frac{d}{d\log\Theta_j}\log \left|x_\alpha\right|,
\end{equation}

\noindent\textbf{Case 1}: $x_\alpha<0$
\begin{eqnarray}
\frac{d}{d\log\Theta_j}\log \left|x_\alpha\right| &=& \frac{1}{\left|x_\alpha\right|} \frac{d}{d\log\Theta_j}\abs{x_\alpha} \\
&=& \frac{-1}{\left|x_\alpha\right|} \frac{d}{d\log\Theta_j}x_\alpha \\
&=& \frac{-1}{\norm{y_\alpha}\cdot\abs{x_\alpha}} \frac{dy(\Theta^\star)_{\alpha}}{d\log\Theta_j},
\end{eqnarray}
\begin{eqnarray}
\frac{d}{d\log\Theta_i}\abs{x_\alpha}^{-1} &=& \frac{1}{\abs{x_\alpha}^2}\frac{d}{d\log\Theta_i}{x_\alpha} \\
&=& \frac{1}{\norm{y_\alpha}\cdot\abs{x_\alpha}^2}\frac{dy(\Theta^\star)_{\alpha}}{d\log\Theta_i},
\end{eqnarray}
consequently
\begin{eqnarray}
\frac{d}{d\log\Theta_i}\frac{d}{d\log\Theta_j}\log \left|x_\alpha\right| &=& \frac{g(x_\alpha)}{\norm{y_\alpha}}\frac{dy(\Theta^\star)_{\alpha}}{d\log\Theta_j}\frac{d}{d\log\Theta_i}\abs{x_\alpha}^{-1} \\
&=& -\frac{1}{\norm{y_\alpha}^2\abs{x_\alpha}^2}\frac{dy(\Theta^\star)_{\alpha}}{d\log\Theta_j}\frac{dy(\Theta^\star)_{\alpha}}{d\log\Theta_i},
\end{eqnarray}

\noindent\textbf{Case 2}: $x_\alpha>0$
\begin{eqnarray}
\frac{d}{d\log\Theta_j}\log \left|x_\alpha\right| &=& \frac{1}{\left|x_\alpha\right|} \frac{d}{d\log\Theta_j}\abs{x_\alpha} \\
&=& \frac{1}{\left|x_\alpha\right|} \frac{d}{d\log\Theta_j}x_\alpha \\
&=& \frac{1}{\norm{y_\alpha}\cdot\abs{x_\alpha}} \frac{dy(\Theta^\star)_{\alpha}}{d\log\Theta_j},
\end{eqnarray}
\begin{eqnarray}
\frac{d}{d\log\Theta_i}\abs{x_\alpha}^{-1} &=& \frac{-1}{\abs{x_\alpha}^2}\frac{d}{d\log\Theta_i}{x_\alpha} \\
&=& \frac{-1}{\norm{y_\alpha}\cdot\abs{x_\alpha}^2}\frac{dy(\Theta^\star)_{\alpha}}{d\log\Theta_i},
\end{eqnarray}

consequently
\begin{eqnarray}
\frac{d}{d\log\Theta_i}\frac{d}{d\log\Theta_j}\log \left|x_\alpha\right| &=& \frac{g(x_\alpha)}{\norm{y_\alpha}}\frac{dy(\Theta^\star)_{\alpha}}{d\log\Theta_j}\frac{d}{d\log\Theta_i}\abs{x_\alpha}^{-1} \\
&=& -\frac{1}{\norm{y_\alpha}^2\abs{x_\alpha}^2}\frac{dy(\Theta^\star)_{\alpha}}{d\log\Theta_j}\frac{dy(\Theta^\star)_{\alpha}}{d\log\Theta_i},
\end{eqnarray}

Such that
\begin{equation}
\frac{d\mathcal{L}(\Theta)}{d\log\Theta_id\log\Theta_j} = \frac{1}{N_S N_K T}\sum_{\alpha} \frac{-1}{\norm{y_\alpha}^2\abs{x_\alpha}^2}\frac{dy(\Theta^\star)_{\alpha}}{d\log\Theta_j}\frac{dy(\Theta^\star)_{\alpha}}{d\log\Theta_i},
\end{equation}

This is different to the normal square loss in two ways:
\begin{enumerate}
    \item There is a $-1$ multiplier for the general second derivative, which means that 
    \item There is an additional re-scaling factor $\abs{x_\alpha}$ which implies that the term within the summation will be of order 1.
\end{enumerate}

\subsection{Approximation with first derivatives ($\mathcal{O}(n)$ operations)}
Taking the first derivative with respect to $\log\Theta_i$, that is with respect to the $i^{th}$ parameter\footnote{
Note that by the chain rule $\frac{dy(\Theta)}{d\Theta_j}=\frac{dy(\Theta)}{d\log\Theta_j}\frac{d\log\Theta_j}{d\Theta_j}$ and thus $\frac{dy(\Theta)}{d\log\Theta_j} = \Theta_j\frac{dy(\Theta)}{d\Theta_j}$
}
\begin{equation}
\frac{d\mathcal{L}(\Theta)}{d\log\Theta_i} = \frac{\Theta_i}{N_S N_K T}\sum_{\alpha}\frac{1}{(\max y_\alpha)^2}\left(y(\Theta)_{\alpha} - y(\Theta^\star)_{\alpha}\right)\frac{dy(\Theta^\star)_{\alpha}}{d\Theta_i},
\end{equation}
we can take the second derivative with respect to $\log\Theta_j$ to yield
\begin{equation}
\frac{d^{2}\mathcal{L}(\Theta)}{d\log\Theta_i d\log\Theta_j} = \frac{\Theta_i\Theta_j}{N_S N_K T}\sum_{\alpha}\frac{1}{(\max y_\alpha)^2}\frac{dy(\Theta^\star)_{\alpha}}{d\Theta_i}\frac{dy(\Theta^\star)_{\alpha}}{d\Theta_j},
\end{equation}
where the second derivative terms fall away because we are evaluating the function at the optimal parameters $\Theta^{\star}$, that is $\frac{d}{d\log\Theta_j}\frac{dy_{s,\alpha}}{d\log\Theta_i}=0$. Numerically, we take the more robust central difference approach to calculating the derivative (step-size $h$). The central difference is the average between an increase and a decrease in the parameter:
\begin{equation}\label{eq:central_difference_derivative}
\frac{dy(\Theta^\star)_{s,\alpha}}{d\log\Theta_i} \approx \frac{y(\log\Theta^{\star} + h e_j)_{s,\alpha} - y(\log\Theta^{\star} - h e_j)_{s,\alpha}}{2h},
\end{equation}

\subsection{Notes on the Order $N$ approximation}
\begin{itemize}
	\item This should guarantee a positive definite matrix to be calculated (useful as a unit test to the analysis of these matrices)
	\item A natural benchmark for the Hessian is thus the Wishart ensemble, whose eigenvalue spectrum would be a $H_0$ hypothesis of randomness 
\end{itemize}

\begin{equation}\label{eq:loss_function}
\mathcal{L}(\Theta) = \frac{1}{2 N_K T}\sum_{k}^{N_K}\sum_{t}^{T}\left(\frac{\mathbb{E}_{s}(y(\Theta)_{k, t}) - \mathbb{E}_{s}(y(\Theta^\star)_{k, t})}{\max y_{i,j}}\right)^2,
\end{equation}

\begin{equation}
\frac{d\mathcal{L}(\Theta)}{d\log\Theta_i} = \frac{\mathbb{E}_{s}(\Theta_i)}{N_K T}\sum_{\alpha}\frac{1}{(\max y_\alpha)^2}\left(\mathbb{E}_{s}(y(\Theta)_{\alpha}) - \mathbb{E}_{s}(y(\Theta^\star)_{\alpha})\right)\frac{d\mathbb{E}_{s}(y(\Theta^\star)_{\alpha})}{d\Theta_i},
\end{equation}

\begin{equation}
\frac{d^{2}\mathcal{L}(\Theta)}{d\log\Theta_i d\log\Theta_j} = \frac{\mathbb{E}_{s}(\Theta_i)\mathbb{E}_{s}(\Theta_j)}{N_K T}\sum_{\alpha}\frac{1}{(\max y_\alpha)^2}\frac{d\mathbb{E}_{s}(y(\Theta^\star)_{\alpha})}{d\Theta_i}\frac{d\mathbb{E}_{s}(y(\Theta^\star)_{\alpha})}{d\Theta_j},
\end{equation}

\begin{equation}
    \frac{d\mathbb{E}_{s}(y(\Theta)_{\alpha})}{d\Theta_i} =\frac{d}{d\Theta_i} \frac{\sum_s y(\Theta)_\alpha}{N_s} = \frac{1}{N_s}\sum_s\frac{dy(\Theta)_\alpha}{d\Theta_i} = \mathbb{E}_s\left(\frac{dy(\Theta)_\alpha}{d\Theta_i}\right)
\end{equation}

\begin{equation}\label{eq:loss_function}
\mathcal{L}(\Theta) = \mathbb{E}_{s}\left(\frac{1}{2 N_K T}\sum_{k}^{N_K}\sum_{t}^{T}\left(\frac{y(\Theta)_{k, t} - y(\Theta^\star)_{k, t}}{\max y_{i,j}}\right)^2\right),
\end{equation}
