# Supplementary material for: Exploration of the Parameter Space in Macroeconomic Agent-Based Models
Source: arXiv:2111.08654 source file (2022-08-05)
Supplement: Supplementary file 5 [file appx_parameters.tex]

\subsection{Summary of Investigations of Gualdi et al (2015) }

\begin{center}
\begin{tabular}{p{1.5cm} p{4cm} p{8cm}} 
 \hline
 Parameter & Description & Finding \\
 \hline\hline\hline
 R                  & Firm: Hiring/firing rate                           & - Fig 4 \\ \hline
 r                  & Firm: adjustment ratio $\frac{\gamma_w}{\gamma_p}$ & - influences average inflation, increase of $\gamma_w$ allows firms to better adapt wages and to absorb the indeptment through inflation (EC shrinks when increasing $\gamma_w$, higher r has a stabilizing effect) \\ \hline
 $\gamma_p$         & Firm: price-adjustment size                        & - Wage dynamics give rise to inflation, influences average inflation \\ \hline
 wage factor        & Firm: wage adjustment to infl.                     & - Wage dynamics give rise to inflation \\ \hline \hline
 $\Theta$           & Bank: Default threshold                            & - strong influence on inflation (high $\Theta$ high infl., low $\Theta$ zero infl., intermediate $\Theta$ defl. and infl.)  \\ \hline
 f                  & Bank: bankruptcy effect on bank interest rates     & - EC can be defanged if HH does not carry the bankruptcies of firms (decreasing f, Fig 6 left 2015) \\ \hline \hline
 $\delta$           & HH: Dividend share                                 & - If $\delta^+$, demand is supported which stabilizes the economy and EC disappears at some point \\ \hline
 $\beta$            & HH: Intensity of choice                            & - increasing $\beta$ increases unemployment, increasing beta is similar to increase $\gamma_p$, savings increase with $\beta$ because HH involuntary save more when they are more selective on prices this reduces avg. price increase and therefore expands the FE region. However, the effect of $\beta$ is numerically very small. \\ \hline

\end{tabular}
\end{center}

\subsection{Summary of Investigations of Gualdi et al (2017) }

\begin{center}
\begin{tabular}{p{1.5cm} p{4cm} p{8cm}} 
 \hline
 Parameter & Description & Finding \\
 \hline\hline\hline
 R                  & Firm: Hiring/firing rate                           & - Turns out to be one of the most important parameter that determine the phase diagram \\ \hline
 $\alpha_\Gamma$    & Firm: loan rate effect on hire/fire                & - If $\alpha_\Gamma = \Gamma_0 = \alpha_c = 0$ then Fig1 is unaffected. The larger $\alpha_\Gamma$ the smaller the critical value $\rho_{**}$ \\ \hline
 $\Gamma_0$         & Firm: baseline $\Gamma$                            & - If $\Gamma_0 = 0$ FE-FU transition is a first order transition, else it is a second order transition. In the good phases $\Gamma_0 \neg 0$ the FE region expands downwards (Fig1) \\ \hline \hline
 $\rho^*$           & CB: baseline interest rate                         & - If $\rho^*$ exceeds inflation rate unemployment increases with $\rho^*$ and inflation decreases. If $\rho^*$ gets larger EC and FE disappear because firms do not want to accumulate more debt and rather reducing their workforce \\ \hline \hline
 $\Theta$           & Bank: Default threshold                            & -  Turns out to be the most important parameter that determine the phase diagram\\ \hline
 f                  & Bank: bankruptcy effect on bank interest rates     & - plays a very little role in the qualitative behaviour of the economy.\\\hline \hline
 $\alpha_c$         & HH: real rate influence on consumption             & - has not a high influence as long as it is chosen within a reasonable range. However for $\Theta > 1$, $\alpha_c$ stabilizes the economy and $R_c$ shifts to lower values with decreasing $\alpha_C$\\ \hline

\end{tabular}
\end{center}
