# Supplementary material for: Exploration of the Parameter Space in Macroeconomic Agent-Based Models
Source: arXiv:2111.08654 source file (2022-08-05)
Supplement: Supplementary file 6 [file lit_review.tex]

\section{Annotated Literature Review}

\subsection{Sloppiness}
General Remarks:
\begin{itemize}
    \item Most systems biology model
\end{itemize}

\noindent \textbf{Specific Literature}:
\begin{enumerate}
    \item \citet{GutenkunstEtAl2007}
    \begin{itemize}
        \item \textbf{Question:}
        \item \textbf{Findings:}
        \item \textbf{Relevance:}
    \end{itemize}
    \item \citet{ApgarEtAl2010}
    \begin{itemize}
        \item \textbf{Question:} How to optimally choose experiments to calibrate a computational model
        \item \textbf{Findings:}
        \begin{enumerate}
            \item Design a method to identify complementary experiments that optimally minimize the parameter uncertainty
            \item Develop experiments that constrain all parameters to within 10\% of their value
            \item Conclusion: parameter uncertainty may not be inherent but can be progressively reduced by perturbation experiments
            \item High precision (e.g. <1\%) tend to require an infeasible amount of experiments (>20)
        \end{enumerate}
        \item \textbf{Relevance:}
        \begin{enumerate}
            \item Notation of determining the set of parameters $\Theta$ that produce an error less that $\chi^2_{\max}$. They have a very concise statement of the Sloppy problem in this way.
            \item Question: what would it mean to do \textit{experiments} in the context of our ABM? Likely the addition of different data sources e.g. different time-series. 
            \item Some methodologically relevant things: (1) normalizing by the standard deviation leads to ML estimator? (2) Thus one can use Cramer-Rao to define lower bound on variance of parameter uncertainty in eigenvector direction, i.e. the ratio of top to bottom in CI around parameters can be computed
        \end{enumerate}
    \end{itemize}
    \item \citet{TranstrumEtAl2010} -- \blue{Very difficult paper, refer to \citet{TranstrumEtAl2011}}
    \begin{itemize}
        \item \textbf{Question:} Explaining the challenge of fitting data by considering a geometric problem
        \item \textbf{Findings:}
        \begin{enumerate}
            \item Multiparameter models are a kind of high-dimensional analytic interpolation scheme, and near degenerate Hessians result whenever multiple data points reside within some generalized radius of convergence.
            \item Fitting difficulties arise due to the narrow boundaries on the model manifold (manifold of predictions in the space of data) with a hierarchy of widths
            \item One can use geodesics to accelerate fitting algorithms to use fewer function evaluations and find the best fit. One can also change the manifold to push the boundaries to 0 or +$\infty$
        \end{enumerate}
        \item \textbf{Relevance:}
        \begin{enumerate}
            \item Not sure for this particular paper - they are more concerned with the fitting process itself (i.e. fitting algorithms), which we are not concerned with for the first paper
        \end{enumerate}
    \end{itemize}
    \item \citet{TranstrumEtAl2011}\red{MSK}
    \begin{itemize}
        \item \textbf{Question: }How to study nonlinear least squares models with a geometric framework?
        \item \textbf{Findings:}
        \begin{enumerate}
            \item Parameters tend to diverge or drift to unphysical values, geometrically corresponding to running off the edge of the manifold. This Problem can be solved by introducing a model graph which is a combination of the model manifold picture and the parameter space picture.
            \item The model’s ‘bare’ parameters are often a poor coordinate choice for the manifold. By constructing alternative coordinates based on geodesic motion, the canyons in the manifold can be transformed into basins.
        \end{enumerate}
        \item \textbf{Relevance:}
        \begin{enumerate}
            \item The approximate Hessian is useful to study the sloppiness of a model independently of the data at points other than the best fit.
            \item  If a region of parameter space has larger eigenvalues by even a small factor, the cumulative effect on the product is that this region of parameter space will occupy most of the model manifold.
        \end{enumerate}
    \end{itemize}
    \item \citet{HagenEtAl2013} -- \blue{Follow-up to \citet{ApgarEtAl2010}}\red{KNW}
    \begin{itemize}
        \item \textbf{Question:} How to select and design experiments to fit the data?
        \item \textbf{Findings:}
        \begin{itemize}
            \item Accurate parameter estimation is achievable with complementary experiments. The resulting parameterized models are capable of accurate predictions.
            \item Spend a lot of time on the 
        \end{itemize}
        \item \textbf{Relevance:}
        \begin{itemize}
            \item They have a more precise mechanic for their experimentation that could be replicated in the future for determining the \textit{optimal} data needed to fit accurately fit all of the ABM's parameters
        \end{itemize}
    \end{itemize}
    \item \citet{MachtaEtAl2013} \red{MSK}
    \begin{itemize}
        \item \textbf{Question: } Do microscopic dependance of emergent theories in physics behave similar than multiparameter models in other areas of science? They examine two models: hopping model of diffusion and ising model of ferromagnetism
        \item \textbf{Findings:} 
        \begin{enumerate}
            \item The sensitivity of model predictions to changes in parameters is quantified by the Fisher Information Matrix (FIM). The FIM forms a metric that converts parameter space distance into a unique measure of distinguishability between a model and nearby model
            \item Calculating the FIM and the respective eigenvalues of the hopping diffusion model for observations after given time steps  show that for more time steps the models eigenvalues span more and more order of magnitudes. The eigenvectors of the biggest eigenvalues describe the physical parameters such as diffusion and drift. The more time elapsed the more difficult it is to measure certain parameters.
            \item Similar behaviour can be seen in the Ising model where the time steps correspond to coarsening the model
        \end{enumerate}
        \item \textbf{Relevance:}
        \begin{enumerate}
            \item Multiparameter models such as in systems biology and other areas of science are sloppy only when fit to experiments that probe collective behavior— if experiments are designed to measure one parameter at a time, no hierarchy can be expected
            \item Few ‘stiff’ eigenvectors in each model point along directions where observables are sensitive to changes in parameters, while progressively sloppier directions make little difference for observables. These sloppy parameters cannot be inferred from data, and conversely, their exact values do not need to be known to quantitatively understand system behavior
        \end{enumerate}
    \end{itemize}
    \item \citet{MourikEtAl2014}
    \begin{itemize}
        \item \textbf{Question:}
        \item \textbf{Findings:}
        \item \textbf{Relevance:}
    \end{itemize}
    \item \citet{Transtrum2014}
    \begin{itemize}
        \item \textbf{Question:}
        \item \textbf{Findings:}
        \item \textbf{Relevance:}
    \end{itemize}
    \item \citet{TranstrumEtAl2015}
    \begin{itemize}
        \item \textbf{Question:}
        \item \textbf{Findings:}
        \item \textbf{Relevance:}
    \end{itemize}
    \item \citet{MannakeeEtAl2016}
    \begin{itemize}
        \item \textbf{Question:}
        \item \textbf{Findings:}
        \item \textbf{Relevance:}
    \end{itemize}
    \item \citet{NiksicVretenar2016}
    \begin{itemize}
        \item \textbf{Question:}
        \item \textbf{Findings:}
        \item \textbf{Relevance:}
    \end{itemize}
    \item \citet{TranstrumQiu2016}
    \begin{itemize}
        \item \textbf{Question:}
        \item \textbf{Findings:}
        \item \textbf{Relevance:}
    \end{itemize}
    \item \citet{WhiteEtAl2016}
    \begin{itemize}
        \item \textbf{Question:}
        \item \textbf{Findings:}
        \item \textbf{Relevance:}
    \end{itemize}
    \item \citet{MacLeod2017}
    \begin{itemize}
        \item \textbf{Question:}
        \item \textbf{Findings:}
        \item \textbf{Relevance:}
    \end{itemize}
    \item \citet{MyasnikovaSpirov2017}
    \begin{itemize}
        \item \textbf{Question:}
        \item \textbf{Findings:}
        \item \textbf{Relevance:}
    \end{itemize}
    \item \citet{RamanEtAl2017}
    \begin{itemize}
        \item \textbf{Question:}
        \item \textbf{Findings:}
        \item \textbf{Relevance:}
    \end{itemize}
    \item \citet{Francis2019}
    \begin{itemize}
        \item \textbf{Question:}
        \item \textbf{Findings:}
        \item \textbf{Relevance:}
    \end{itemize}
    \item \citet{Quinn2019}
    \begin{itemize}
        \item \textbf{Question:}
        \item \textbf{Findings:}
        \item \textbf{Relevance:}
    \end{itemize}
    \item \citet{Villaverde2019}
    \begin{itemize}
        \item \textbf{Question:}
        \item \textbf{Findings:}
        \item \textbf{Relevance:}
    \end{itemize}
    \item \citet{HsuEtAl2020}
    \begin{itemize}
        \item \textbf{Question:}
        \item \textbf{Findings:}
        \item \textbf{Relevance:}
    \end{itemize}
    \item \citet{Ligmann-ZielinskaEtAl2020}
\end{enumerate}

\subsection{Macroeconomic ABM Metamodeling \& co (Counterpart literature)}
There are a lot of studies on meta-modeling and sensitivity analysis. Their aim is to give an indication of which parameters the model is sensitive to w.r.t some summary statistics. However, they do so across the entirety of the solution space. Nor has there been a study of the parameter uncertainty.
\begin{enumerate}
    \item \citet{SalleYildizoglu2014}
    \begin{itemize}
        \item \textbf{Question:}
        \item \textbf{Findings:}
        \item \textbf{Relevance:}
    \end{itemize}
    \item \citet{LampertiEtAl2018}
    \begin{itemize}
        \item \textbf{Question:}
        \item \textbf{Findings:}
        \item \textbf{Relevance:}
    \end{itemize}
    \item \citet{vanderHoog2019}
    \begin{itemize}
        \item \textbf{Question:}
        \item \textbf{Findings:}
        \item \textbf{Relevance:}
    \end{itemize}
    \item \citet{BargigliEtAl2020}
    \begin{itemize}
        \item \textbf{Question:}
        \item \textbf{Findings:}
        \item \textbf{Relevance:}
    \end{itemize}
    \item \citet{ZhangEtAl2020}
    \begin{itemize}
        \item \textbf{Question:}
        \item \textbf{Findings:}
        \item \textbf{Relevance:}
    \end{itemize}
    \item \citet{ChenDesiderio2021}
    \begin{itemize}
        \item \textbf{Question:}
        \item \textbf{Findings:}
        \item \textbf{Relevance:}
    \end{itemize}
    \item \citet{Platt2021}
    \begin{itemize}
        \item \textbf{Question:}
        \item \textbf{Findings:}
        \item \textbf{Relevance:}
    \end{itemize}
    \item \citet{RoblesEtAl2021}
    \begin{itemize}
        \item \textbf{Question:}
        \item \textbf{Findings:}
        \item \textbf{Relevance:}
    \end{itemize}
    \item \citet{tenBroekeEtAl2021}
\end{enumerate}
