# Supplementary material for: Exploration of the Parameter Space in Macroeconomic Agent-Based Models
Source: arXiv:2111.08654 source file (2022-08-05)
Supplement: Supplementary file 7 [file notes.tex]

exponentials (akin to nuclear decay). Consider the function
\begin{equation}\label{eq:exponential_function}
    f(t, \Theta) = \sum_{k=1}^K A_ke^{-\gamma_kt},
\end{equation}
with parameter vector $\Theta=[A_1, \dots, A_K, \gamma_1, \dots, \gamma_K]$ where $\gamma_k, A_k>0~\forall K$.

We consider the loss function of Eq. \eqref{eq:loss_function} in the absence of noise ($N_s=1$), and for only one variable ($N_k=1$):
\begin{equation}\label{eq:exponential_loss_function}
\mathcal{L}(\Theta) = \frac{1}{2T}\sum_{t}^{T}\left(
f(t,\Theta) - f(t,\Theta^\star)
%\frac{f(t,\Theta) - f(t,\Theta^\star)}{\max_t f(\Theta^\star)}
\right)^2,
\end{equation}
as a simplification of the original noise function that will allow us to demonstrate the feasibility of our numerical estimates. 

From this we can then derive the Hessian matrix that will be numerically approximated as
\begin{equation}
H_{i,j}^{\mathcal{L}} \equiv \frac{d^2\mathcal{L}}{d\Theta_i d\Theta_j}
\end{equation}
at the point $\Theta^\star$ by taking the second derivative at this point
\begin{equation}
\frac{d\mathcal{L}(\Theta)}{d\Theta_i} = \frac{1}{T%\max_t f(\Theta^\star)
}\sum_{T}\left(f(t, \Theta) - f(t, \Theta^\star)\right)\frac{df(t, \Theta^\star)}{d\Theta_i},
\end{equation}
\begin{equation}
\frac{d^2\mathcal{L}(\Theta)}{d\Theta_i d\Theta_j} = \frac{1}{T%\max_t f(\Theta^\star)
}\sum_{T}\frac{df(t, \Theta^\star)}{d\Theta_i}\frac{df(t, \Theta^\star)}{d\Theta_j},
\end{equation} 

From an analytical standpoint, we know that the vector of $\frac{df(t, \Theta^\star)}{d\Theta_i}$ is the Jacobian, $J$, which is 
\begin{equation}
    J = 
    \left[\begin{array}{c}
         e^{-\gamma_1t} \\
         \vdots \\
         e^{-\gamma_Kt} \\
         -A_1te^{-\gamma_1t} \\
         \vdots \\
         -A_Kte^{-\gamma_Kt} \\
    \end{array}\right],
\end{equation}
which leads us to the analytical Hessian Matrix $H^\star$ for the case of $K=2$
\begin{equation}
    H^\star = \frac{1}{T}\sum_{T}\left[\begin{array}{cccc}
        e^{-2\gamma_1t} & e^{-(\gamma_1 + \gamma_2)t} & -A_1te^{-2\gamma_1t} & -A_1te^{-(\gamma_1 + \gamma_2)t} \\
        
        e^{-(\gamma_2 + \gamma_1)t} & e^{-2\gamma_2t} & -A_2te^{-(\gamma_2 + \gamma_1)t} & -A_2te^{-2\gamma_2t} \\

        -A_1te^{-2\gamma_1t} & -A_1te^{-(\gamma_1 + \gamma_2)t} & A_1^2t^2e^{-2\gamma_1t} & A_1A_2t^2e^{-(\gamma_1 + \gamma_2)t} \\
        -A_2te^{-(\gamma_2 + \gamma_1)t} & -A_2te^{-2\gamma_2t} & A_1A_2t^2e^{-(\gamma_1 + \gamma_2)t} & A_2^2t^2e^{-2\gamma_2} \\

    \end{array}\right]
\end{equation}
