# Supplementary material for: Exploration of the Parameter Space in Macroeconomic Agent-Based Models
Source: arXiv:2111.08654 source file (2022-08-05)
Supplement: Supplementary file 8 [file appx_first_order_approx.tex]

\subsection{Definition of the loss function}
Parameter set $\Theta$, with target set $\Theta^{\star}$ generates a time-series realisation of $k\in\{1,\dots,N_K\}$ variables over $t\in\{1,\dots,T\}$ periods using the random seeds $s\in\{1,\dots,N_S\}$

\begin{equation}\label{eq:loss_function}
\mathcal{L}(\Theta) = \frac{1}{2N_S N_K T}\sum_{s}^{N_S}\sum_{k}^{N_K}\sum_{t}^{T}\left(\frac{y(\Theta)_{s, k, t} - y(\Theta^\star)_{s, k, t}}{\max y_{i,j}}\right)^2,
\end{equation}

\begin{equation}\label{eq:loss_function}
\mathcal{L}(\Theta) = \frac{1}{2N_S N_K T}\sum_{s}^{N_S}\sum_{k}^{N_K}\sum_{t}^{T}\left(\frac{y(\Theta^\star)_{s, k, t} - y(\Theta)_{s, k, t}}{y(\Theta^\star)_{s, k, t}}\right)^2 = \frac{1}{2N_S N_K T}\sum_{s}^{N_S}\sum_{k}^{N_K}\sum_{t}^{T}\left(1 - \frac{y(\Theta)_{s, k, t}}{y(\Theta^\star)_{s, k, t}}\right)^2,
\end{equation}

where we can introduce $\alpha=(s,k,t)$ to simplify the summation to

\begin{equation}\label{eq:loss_function_simple}
\mathcal{L}(\Theta) = \frac{1}{2N_S N_K T}\sum_{\alpha}\frac{1}{(\max y_\alpha)^2}\left(y(\Theta)_{\alpha} - y(\Theta^\star)_{\alpha}\right)^2,
\end{equation}

\subsection{The Hessian Matrix}
The Hessian matrix is defined as the matrix of second derivates, whose $(i,j)$ entry is the cross derivative of the $i^{th}$ and $j^{th}$ parameter is defined by
\begin{equation}
H_{j,k}^{\mathcal{L}} \equiv \frac{d^2\mathcal{L}}{d\log\Theta_i d\log\Theta_j}
\end{equation}
Here, the derivative is taken with respect to the natural logarithm of $\Theta_i$ to account for parameters with different order of magnitudes. The Hessian can be directly numerically estimated by an $\mathcal{O}(n^2)$ via:

\subsection{Approximation with first derivatives ($\mathcal{O}(n)$ operations)}
Taking the first derivative with respect to $\log\Theta_i$, that is with respect to the $i^{th}$ parameter\footnote{
Note that by the chain rule $\frac{dy(\Theta)}{d\Theta_j}=\frac{dy(\Theta)}{d\log\Theta_j}\frac{d\log\Theta_j}{d\Theta_j}$ and thus $\frac{dy(\Theta)}{d\log\Theta_j} = \Theta_j\frac{dy(\Theta)}{d\Theta_j}$
}
\begin{equation}
\frac{d\mathcal{L}(\Theta)}{d\log\Theta_i} = \frac{\Theta_i}{N_S N_K T}\sum_{\alpha}\frac{1}{(\max y_\alpha)^2}\left(y(\Theta)_{\alpha} - y(\Theta^\star)_{\alpha}\right)\frac{dy(\Theta^\star)_{\alpha}}{d\Theta_i},
\end{equation}
we can take the second derivative with respect to $\log\Theta_j$ to yield
\begin{equation}
\frac{d^{2}\mathcal{L}(\Theta)}{d\log\Theta_i d\log\Theta_j} = \frac{\Theta_i\Theta_j}{N_S N_K T}\sum_{\alpha}\frac{1}{(\max y_\alpha)^2}\frac{dy(\Theta^\star)_{\alpha}}{d\Theta_i}\frac{dy(\Theta^\star)_{\alpha}}{d\Theta_j},
\end{equation}
where the second derivative terms fall away because we are evaluating the function at the optimal parameters $\Theta^{\star}$, that is $\frac{d}{d\log\Theta_j}\frac{dy_{s,\alpha}}{d\log\Theta_i}=0$. Numerically, we take the more robust central difference approach to calculating the derivative (step-size $h$). The central difference is the average between an increase and a decrease in the parameter:
\begin{equation}\label{eq:central_difference_derivative}
\frac{dy(\Theta^\star)_{s,\alpha}}{d\log\Theta_i} \approx \frac{y(\log\Theta^{\star} + h e_j)_{s,\alpha} - y(\log\Theta^{\star} - h e_j)_{s,\alpha}}{2h},
\end{equation}

\subsection{Notes on the Order $N$ approximation}
\begin{itemize}
	\item This should guarantee a positive definite matrix to be calculated (useful as a unit test to the analysis of these matrices)
	\item A natural benchmark for the Hessian is thus the Wishart ensemble, whose eigenvalue spectrum would be a $H_0$ hypothesis of randomness 
\end{itemize}

\begin{equation}\label{eq:loss_function}
\mathcal{L}(\Theta) = \frac{1}{2 N_K T}\sum_{k}^{N_K}\sum_{t}^{T}\left(\frac{\mathbb{E}_{s}(y(\Theta)_{k, t}) - \mathbb{E}_{s}(y(\Theta^\star)_{k, t})}{\max y_{i,j}}\right)^2,
\end{equation}

\begin{equation}
\frac{d\mathcal{L}(\Theta)}{d\log\Theta_i} = \frac{\mathbb{E}_{s}(\Theta_i)}{N_K T}\sum_{\alpha}\frac{1}{(\max y_\alpha)^2}\left(\mathbb{E}_{s}(y(\Theta)_{\alpha}) - \mathbb{E}_{s}(y(\Theta^\star)_{\alpha})\right)\frac{d\mathbb{E}_{s}(y(\Theta^\star)_{\alpha})}{d\Theta_i},
\end{equation}

\begin{equation}
\frac{d^{2}\mathcal{L}(\Theta)}{d\log\Theta_i d\log\Theta_j} = \frac{\mathbb{E}_{s}(\Theta_i)\mathbb{E}_{s}(\Theta_j)}{N_K T}\sum_{\alpha}\frac{1}{(\max y_\alpha)^2}\frac{d\mathbb{E}_{s}(y(\Theta^\star)_{\alpha})}{d\Theta_i}\frac{d\mathbb{E}_{s}(y(\Theta^\star)_{\alpha})}{d\Theta_j},
\end{equation}

\begin{equation}
    \frac{d\mathbb{E}_{s}(y(\Theta)_{\alpha})}{d\Theta_i} =\frac{d}{d\Theta_i} \frac{\sum_s y(\Theta)_\alpha}{N_s} = \frac{1}{N_s}\sum_s\frac{dy(\Theta)_\alpha}{d\Theta_i} = \mathbb{E}_s\left(\frac{dy(\Theta)_\alpha}{d\Theta_i}\right)
\end{equation}

\begin{equation}\label{eq:loss_function}
\mathcal{L}(\Theta) = \mathbb{E}_{s}\left(\frac{1}{2 N_K T}\sum_{k}^{N_K}\sum_{t}^{T}\left(\frac{y(\Theta)_{k, t} - y(\Theta^\star)_{k, t}}{\max y_{i,j}}\right)^2\right),
\end{equation}
